# Supplementary material for: RDF Translator: A RESTful Multi-Format Data Converter for the Semantic Web
Source: arXiv:1312.4704 source file (2013-12-17)
Supplement: Supplementary file 1 [file rdf-translator-6-appendix.tex]

%% rdf-translator-6-appendix.tex

\appendix

\section{RDF Distiller Test}

Scenario:
Extracted N3 from http://www.stalsoft.com/
Tried to convert N3 output to RDF/XML

\begin{lstlisting}
RDF::ReaderError: 
     vcard:postal-code "85579"@en^^xsd:string;

---------------------------------^
Error on line 54 at offset 33: Found '^^' when parsing a pathtail. expected  | "!","expression" | "^","expression"
\end{lstlisting}

error messages are quite verbose, but the converter should not generate typed language literals.
